# Supplementary material for: Decentralized Safe Reinforcement Learning for Voltage Control
Source: arXiv:2110.01126 source file (2021-10-03)
Supplement: Supplementary file 1 [file appendix.tex]

% \subsection{Preliminary Lemma}

% \subsection{Proof of Theorem~\ref{theorem:stable}}
% \begin{proof}
% Let $E(\bm{v}_t) = \bm{v}_t^{T}\mathbf{X}^{-1}\bm{v}_t$ be a control Lyapunov function for the system. Then $\Delta E(\bm{v}_{t})=E(\bm{v}_{t+1})-E(\bm{v}_{t}) =  -2 \bm{v}_t^T\bm{u}_t+\bm{u}_t^T\mathbf{X}\bm{u}_t$. From Lyapunov stability theory, if $E(\bm{v}_{t+1})-E(\bm{v}_{t})<0$ for all $t$, then the system is asymptotically stable. 


% Since $\frac{\bm{u}_t^T\mathbf{X}\bm{u}_t}{\bm{u}_t^T\bm{u}_t}\leq \lambda_{max}(\mathbf{X})$, we have  $\Delta E(\bm{v}_{t})\leq -2 \bm{v}_t^T\bm{u}_t+\lambda_{max}(\mathbf{X})\bm{u}_t^T\bm{u}_t$. Suppose $u_i(v_i)$ is the same sign as $v_i$ and $|u_i(v_i)|< \frac{2}{\lambda_{max}(\mathbf{\mathbf{X}})}|v_i| $ for all $i=1,\cdots,N$, then we have $-2\bm{v}_t^T\bm{u}_t< -\lambda_{max}(\mathbf{X})\bm{u}_t^T\bm{u}_t$. Therefore, $\Delta E(\bm{v}_{t})<0$.


% By the Krasovski-Lasalle principle~\cite{aastrom2010feedback}, the constraint on control action can be further relaxed to include equality, i.e.,  $|u_i(v_i)|\leq \frac{2}{\lambda_{max}(\mathbf{X})}|v_i| $ for all $i=1,\cdots,N$. Define the set $S=\left\{\bm{v}_{t}: \Delta E(\bm{v}_{t})=0\right\}$.  If $\bm{v_{t}}\neq 0$ and $|\bm{u}_t|= \frac{2}{\lambda_{max}(\mathbf{X})}|\bm{v_{t}}|$, then $\bm{v_{t+1}}\neq \bm{v_{t}}$ and the operating point is not in the invariant set of the system. Therefore, $S$ contains no invariant sets other than the states that $\bm{v_{t}}=0$.  

% Next we show the part about exponential stability. 
% The Jacobian of the state transition dynamics~\eqref{eq:reduced_transition} is 
% \begin{equation}\label{eq:jacobian}
%     \mathbf{J}(\bm{v})=\mathbf{I}-\mathbf{X}\nabla_{\bm{v}}\bm{u}
% \end{equation}
% where $\nabla_{\bm{v}}\bm{u}$ is the gradient of control action $\bm{u}$ with respect to $\bm{v}$ defined as
% \begin{equation}\label{eq:J_v_w}
% \nabla_{\bm{v}}\bm{u}=
% \begin{bmatrix}
% \begin{smallmatrix}
%     \frac{\mathrm{d}u_1(v_1) }{\mathrm{d} v_1} & & \\
%     & \ddots & \\
%     & & \frac{\mathrm{d}u_{N}(v_{N}) }{\mathrm{d} v_{N}} 
% \end{smallmatrix}
% \end{bmatrix}
% \end{equation}
% From Lemma~\ref{lemma: eigenvalue}, the eigenvalue of $\mathbf{J}(\bm{v})$ is the same as $\mathbf{I}-(\nabla_{\bm{v}}\bm{u})^{\frac{1}{2}}\mathbf{X}(\nabla_{\bm{v}}\bm{u})^{\frac{1}{2}}$.

% From $0 \prec \nabla_{\bm{v}}\bm{u} \prec 2\mathbf{X}^{-1}$ and $\mathbf{X}\succ 0$, we have $(\nabla_{\bm{v}}\bm{u})^{-1} \succ  \frac{1}{2}\mathbf{X}$. Since  $\nabla_{\bm{v}}\bm{u}\succ 0$ is diagonal, we then have $(\nabla_{\bm{v}}\bm{u})^{\frac{1}{2}}\mathbf{X}(\nabla_{\bm{v}}\bm{u})^{\frac{1}{2}} \prec 2\mathbf{I}$ and thus $-\mathbf{I}\prec \mathbf{I}-(\nabla_{\bm{v}}\bm{u})^{\frac{1}{2}}\mathbf{X}(\nabla_{\bm{v}}\bm{u})^{\frac{1}{2}}\prec \mathbf{I}$. The right side inequality holds because $\mathbf{X}\succ 0$.


% Therefore,  the eigenvalue of $\mathbf{J}(\bm{v})$ is strictly smaller than 1, which is equivalent to an exponentially stable system around the equilibrium.
% \end{proof}
